# Supplementary material for: How to Fine-tune Models with Few Samples: Update, Data Augmentation, and Test-time Augmentation
Source: arXiv:2205.07874 source file (2022-08-19)
Supplement: Supplementary file 1 [file legacy.tex]

% and \ref{fig:v_measure_tiered}: ResNet18 pre-trained on tieredImageNet, respectively.

% % ; more red dots are placed above the $y=x$ line.
% % This shows that clustering ability of the feature extractor improves by more samples for FT. 

% \begin{figure}[h!]
% \centering
%      \begin{subfigure}[h]{0.24\linewidth}
%          \includegraphics[width=\linewidth]{figure/v_score/mini/1shot_mini_test.pdf}
%      \end{subfigure}
%      \begin{subfigure}[h]{0.24\linewidth}
%          \includegraphics[width=\linewidth]{figure/v_score/mini/5shot_mini_test.pdf}
%      \end{subfigure}
%     %  \begin{subfigure}[h]{0.24\linewidth}
%     %      \includegraphics[width=\linewidth]{figure/v_score/mini/10shot_mini_test.pdf}
%     %  \end{subfigure}
%      \begin{subfigure}[h]{0.24\linewidth}
%          \includegraphics[width=\linewidth]{figure/v_score/mini/20shot_mini_test.pdf}
%      \end{subfigure}
     
     
%      \begin{subfigure}[h]{0.24\linewidth}
%          \includegraphics[width=\linewidth]{figure/v_score/mini/1shot_tiered_test.pdf}
%      \end{subfigure}
%      \begin{subfigure}[h]{0.24\linewidth}
%          \includegraphics[width=\linewidth]{figure/v_score/mini/5shot_tiered_test.pdf}
%      \end{subfigure}
%     %  \begin{subfigure}[h]{0.24\linewidth}
%     %      \includegraphics[width=\linewidth]{figure/v_score/mini/10shot_tiered_test.pdf}
%     %  \end{subfigure}
%      \begin{subfigure}[h]{0.24\linewidth}
%          \includegraphics[width=\linewidth]{figure/v_score/mini/20shot_tiered_test.pdf}
%      \end{subfigure}
     
%      \begin{subfigure}[h]{0.24\linewidth}
%          \includegraphics[width=\linewidth]{figure/v_score/mini/1shot_places.pdf}
%      \end{subfigure}
%      \begin{subfigure}[h]{0.24\linewidth}
%          \includegraphics[width=\linewidth]{figure/v_score/mini/5shot_places.pdf}
%      \end{subfigure}
%     %  \begin{subfigure}[h]{0.24\linewidth}
%     %      \includegraphics[width=\linewidth]{figure/v_score/mini/10shot_places.pdf}
%     %  \end{subfigure}
%      \begin{subfigure}[h]{0.24\linewidth}
%          \includegraphics[width=\linewidth]{figure/v_score/mini/20shot_places.pdf}
%      \end{subfigure}
     
%       \begin{subfigure}[h]{0.24\linewidth}
%          \includegraphics[width=\linewidth]{figure/v_score/mini/1shot_plantae.pdf}
%      \end{subfigure}
%      \begin{subfigure}[h]{0.24\linewidth}
%          \includegraphics[width=\linewidth]{figure/v_score/mini/5shot_plantae.pdf}
%      \end{subfigure}
%     %  \begin{subfigure}[h]{0.24\linewidth}
%     %      \includegraphics[width=\linewidth]{figure/v_score/mini/10shot_plantae.pdf}
%     %  \end{subfigure}
%      \begin{subfigure}[h]{0.24\linewidth}
%          \includegraphics[width=\linewidth]{figure/v_score/mini/20shot_plantae.pdf}
%      \end{subfigure}
     
%      \begin{subfigure}[h]{0.24\linewidth}
%          \includegraphics[width=\linewidth]{figure/v_score/mini/1shot_cars.pdf}
%      \end{subfigure}
%      \begin{subfigure}[h]{0.24\linewidth}
%          \includegraphics[width=\linewidth]{figure/v_score/mini/5shot_cars.pdf}
%      \end{subfigure}
%     %  \begin{subfigure}[h]{0.24\linewidth}
%     %      \includegraphics[width=\linewidth]{figure/v_score/mini/10shot_cars.pdf}
%     %  \end{subfigure}
%      \begin{subfigure}[h]{0.24\linewidth}
%          \includegraphics[width=\linewidth]{figure/v_score/mini/20shot_cars.pdf}
%      \end{subfigure}
     
%      \begin{subfigure}[h]{0.24\linewidth}
%          \includegraphics[width=\linewidth]{figure/v_score/mini/1shot_cub.pdf}
%      \end{subfigure}
%      \begin{subfigure}[h]{0.24\linewidth}
%          \includegraphics[width=\linewidth]{figure/v_score/mini/5shot_cub.pdf}
%      \end{subfigure}
%     %  \begin{subfigure}[h]{0.24\linewidth}
%     %      \includegraphics[width=\linewidth]{figure/v_score/mini/10shot_cub.pdf}
%     %  \end{subfigure}
%      \begin{subfigure}[h]{0.24\linewidth}
%          \includegraphics[width=\linewidth]{figure/v_score/mini/20shot_cub.pdf}
%      \end{subfigure}
     
%       \begin{subfigure}[h]{0.24\linewidth}
%          \includegraphics[width=\linewidth]{figure/v_score/mini/1shot_crop.pdf}
%      \end{subfigure}
%      \begin{subfigure}[h]{0.24\linewidth}
%          \includegraphics[width=\linewidth]{figure/v_score/mini/5shot_crop.pdf}
%      \end{subfigure}
%     %  \begin{subfigure}[h]{0.24\linewidth}
%     %      \includegraphics[width=\linewidth]{figure/v_score/mini/10shot_crop.pdf}
%     %  \end{subfigure}
%      \begin{subfigure}[h]{0.24\linewidth}
%          \includegraphics[width=\linewidth]{figure/v_score/mini/20shot_crop.pdf}
%      \end{subfigure}
     
%      \begin{subfigure}[h]{0.24\linewidth}
%          \includegraphics[width=\linewidth]{figure/v_score/mini/1shot_euro.pdf}
%      \end{subfigure}
%      \begin{subfigure}[h]{0.24\linewidth}
%          \includegraphics[width=\linewidth]{figure/v_score/mini/5shot_euro.pdf}
%      \end{subfigure}
%     %  \begin{subfigure}[h]{0.24\linewidth}
%     %      \includegraphics[width=\linewidth]{figure/v_score/mini/10shot_euro.pdf}
%     %  \end{subfigure}
%      \begin{subfigure}[h]{0.24\linewidth}
%          \includegraphics[width=\linewidth]{figure/v_score/mini/20shot_euro.pdf}
%      \end{subfigure}
     
%      \begin{subfigure}[h]{0.24\linewidth}
%          \includegraphics[width=\linewidth]{figure/v_score/mini/1shot_isic.pdf}
%      \end{subfigure}
%      \begin{subfigure}[h]{0.24\linewidth}
%          \includegraphics[width=\linewidth]{figure/v_score/mini/5shot_isic.pdf}
%      \end{subfigure}
%     %  \begin{subfigure}[h]{0.24\linewidth}
%     %      \includegraphics[width=\linewidth]{figure/v_score/mini/10shot_isic.pdf}
%     %  \end{subfigure}
%      \begin{subfigure}[h]{0.24\linewidth}
%          \includegraphics[width=\linewidth]{figure/v_score/mini/20shot_isic.pdf}
%      \end{subfigure}
     
     
%       \begin{subfigure}[h]{0.24\linewidth}
%          \includegraphics[width=\linewidth]{figure/v_score/mini/1shot_chest.pdf}
%      \end{subfigure}
%      \begin{subfigure}[h]{0.24\linewidth}
%          \includegraphics[width=\linewidth]{figure/v_score/mini/5shot_chest.pdf}
%      \end{subfigure}
%     %  \begin{subfigure}[h]{0.24\linewidth}
%     %      \includegraphics[width=\linewidth]{figure/v_score/mini/10shot_chest.pdf}
%     %  \end{subfigure}
%      \begin{subfigure}[h]{0.24\linewidth}
%          \includegraphics[width=\linewidth]{figure/v_score/mini/20shot_chest.pdf}
%      \end{subfigure}
%      \caption{Feature extractor’s clustering ability by V-measure and performance differences between LP and FT. The pre-trained model is ResNet10 on miniIN.} \label{fig:v_measure_miniIN}
% \end{figure}

% % \begin{figure}[h!]
% % \centering
% %      \begin{subfigure}[h]{0.255\linewidth}
% %          \includegraphics[width=\linewidth]{figure/v_score/tiered/1shot_mini_test.pdf}
% %      \end{subfigure}
% %      \begin{subfigure}[h]{0.23\linewidth}
% %          \includegraphics[width=\linewidth]{figure/v_score/tiered/5shot_mini_test.pdf}
% %      \end{subfigure}
% %      \begin{subfigure}[h]{0.23\linewidth}
% %          \includegraphics[width=\linewidth]{figure/v_score/tiered/10shot_mini_test.pdf}
% %      \end{subfigure}
% %      \begin{subfigure}[h]{0.23\linewidth}
% %          \includegraphics[width=\linewidth]{figure/v_score/tiered/20shot_mini_test.pdf}
% %      \end{subfigure}
     
     
% %      \begin{subfigure}[h]{0.255\linewidth}
% %          \includegraphics[width=\linewidth]{figure/v_score/tiered/1shot_tiered_test.pdf}
% %      \end{subfigure}
% %      \begin{subfigure}[h]{0.23\linewidth}
% %          \includegraphics[width=\linewidth]{figure/v_score/tiered/5shot_tiered_test.pdf}
% %      \end{subfigure}
% %      \begin{subfigure}[h]{0.23\linewidth}
% %          \includegraphics[width=\linewidth]{figure/v_score/tiered/10shot_tiered_test.pdf}
% %      \end{subfigure}
% %      \begin{subfigure}[h]{0.23\linewidth}
% %          \includegraphics[width=\linewidth]{figure/v_score/tiered/20shot_tiered_test.pdf}
% %      \end{subfigure}
     
% %      \begin{subfigure}[h]{0.255\linewidth}
% %          \includegraphics[width=\linewidth]{figure/v_score/tiered/1shot_places.pdf}
% %      \end{subfigure}
% %      \begin{subfigure}[h]{0.23\linewidth}
% %          \includegraphics[width=\linewidth]{figure/v_score/tiered/5shot_places.pdf}
% %      \end{subfigure}
% %      \begin{subfigure}[h]{0.23\linewidth}
% %          \includegraphics[width=\linewidth]{figure/v_score/tiered/10shot_places.pdf}
% %      \end{subfigure}
% %      \begin{subfigure}[h]{0.23\linewidth}
% %          \includegraphics[width=\linewidth]{figure/v_score/tiered/20shot_places.pdf}
% %      \end{subfigure}
     
% %       \begin{subfigure}[h]{0.255\linewidth}
% %          \includegraphics[width=\linewidth]{figure/v_score/tiered/1shot_plantae.pdf}
% %      \end{subfigure}
% %      \begin{subfigure}[h]{0.23\linewidth}
% %          \includegraphics[width=\linewidth]{figure/v_score/tiered/5shot_plantae.pdf}
% %      \end{subfigure}
% %      \begin{subfigure}[h]{0.23\linewidth}
% %          \includegraphics[width=\linewidth]{figure/v_score/tiered/10shot_plantae.pdf}
% %      \end{subfigure}
% %      \begin{subfigure}[h]{0.23\linewidth}
% %          \includegraphics[width=\linewidth]{figure/v_score/tiered/20shot_plantae.pdf}
% %      \end{subfigure}
     
% %      \begin{subfigure}[h]{0.255\linewidth}
% %          \includegraphics[width=\linewidth]{figure/v_score/tiered/1shot_cars.pdf}
% %      \end{subfigure}
% %      \begin{subfigure}[h]{0.23\linewidth}
% %          \includegraphics[width=\linewidth]{figure/v_score/tiered/5shot_cars.pdf}
% %      \end{subfigure}
% %      \begin{subfigure}[h]{0.23\linewidth}
% %          \includegraphics[width=\linewidth]{figure/v_score/tiered/10shot_cars.pdf}
% %      \end{subfigure}
% %      \begin{subfigure}[h]{0.23\linewidth}
% %          \includegraphics[width=\linewidth]{figure/v_score/tiered/20shot_cars.pdf}
% %      \end{subfigure}
     
% %      \begin{subfigure}[h]{0.255\linewidth}
% %          \includegraphics[width=\linewidth]{figure/v_score/tiered/1shot_cub.pdf}
% %      \end{subfigure}
% %      \begin{subfigure}[h]{0.23\linewidth}
% %          \includegraphics[width=\linewidth]{figure/v_score/tiered/5shot_cub.pdf}
% %      \end{subfigure}
% %      \begin{subfigure}[h]{0.23\linewidth}
% %          \includegraphics[width=\linewidth]{figure/v_score/tiered/10shot_cub.pdf}
% %      \end{subfigure}
% %      \begin{subfigure}[h]{0.23\linewidth}
% %          \includegraphics[width=\linewidth]{figure/v_score/tiered/20shot_cub.pdf}
% %      \end{subfigure}
     
% %       \begin{subfigure}[h]{0.255\linewidth}
% %          \includegraphics[width=\linewidth]{figure/v_score/tiered/1shot_crop.pdf}
% %      \end{subfigure}
% %      \begin{subfigure}[h]{0.23\linewidth}
% %          \includegraphics[width=\linewidth]{figure/v_score/tiered/5shot_crop.pdf}
% %      \end{subfigure}
% %      \begin{subfigure}[h]{0.23\linewidth}
% %          \includegraphics[width=\linewidth]{figure/v_score/tiered/10shot_crop.pdf}
% %      \end{subfigure}
% %      \begin{subfigure}[h]{0.23\linewidth}
% %          \includegraphics[width=\linewidth]{figure/v_score/tiered/20shot_crop.pdf}
% %      \end{subfigure}
     
% %      \begin{subfigure}[h]{0.255\linewidth}
% %          \includegraphics[width=\linewidth]{figure/v_score/tiered/1shot_euro.pdf}
% %      \end{subfigure}
% %      \begin{subfigure}[h]{0.23\linewidth}
% %          \includegraphics[width=\linewidth]{figure/v_score/tiered/5shot_euro.pdf}
% %      \end{subfigure}
% %      \begin{subfigure}[h]{0.23\linewidth}
% %          \includegraphics[width=\linewidth]{figure/v_score/tiered/10shot_euro.pdf}
% %      \end{subfigure}
% %      \begin{subfigure}[h]{0.23\linewidth}
% %          \includegraphics[width=\linewidth]{figure/v_score/tiered/20shot_euro.pdf}
% %      \end{subfigure}
     
% %      \begin{subfigure}[h]{0.255\linewidth}
% %          \includegraphics[width=\linewidth]{figure/v_score/tiered/1shot_isic.pdf}
% %      \end{subfigure}
% %      \begin{subfigure}[h]{0.23\linewidth}
% %          \includegraphics[width=\linewidth]{figure/v_score/tiered/5shot_isic.pdf}
% %      \end{subfigure}
% %      \begin{subfigure}[h]{0.23\linewidth}
% %          \includegraphics[width=\linewidth]{figure/v_score/tiered/10shot_isic.pdf}
% %      \end{subfigure}
% %      \begin{subfigure}[h]{0.23\linewidth}
% %          \includegraphics[width=\linewidth]{figure/v_score/tiered/20shot_isic.pdf}
% %      \end{subfigure}
     
     
% %       \begin{subfigure}[h]{0.255\linewidth}
% %          \includegraphics[width=\linewidth]{figure/v_score/tiered/1shot_chest.pdf}
% %      \end{subfigure}
% %      \begin{subfigure}[h]{0.23\linewidth}
% %          \includegraphics[width=\linewidth]{figure/v_score/tiered/5shot_chest.pdf}
% %      \end{subfigure}
% %      \begin{subfigure}[h]{0.23\linewidth}
% %          \includegraphics[width=\linewidth]{figure/v_score/tiered/10shot_chest.pdf}
% %      \end{subfigure}
% %      \begin{subfigure}[h]{0.23\linewidth}
% %          \includegraphics[width=\linewidth]{figure/v_score/tiered/20shot_chest.pdf}
% %      \end{subfigure}
% %      \caption{Feature extractor’s clustering ability by V-measure and performance differences between LP and FT. The pre-trained model is ResNet10 on miniIN.} \label{fig:v_measure_tiered}
% % \end{figure}





% Table \ref{tab:miniIN_1_shot_da} shows the 5-way $k$-shot performance according to data augmentation techniques for $k \in \{1, 5, 20\}$. 

% \begin{table}[h!]
%     \centering
%     \resizebox{\linewidth}{!}{
%     %\vskip 0.10in
%     \begin{tabular}{lccccc}
%     \toprule
%     \multicolumn{6}{l}{$k$ = 1} \\ \midrule
%     Aug. & miniIN & \!\!\!tieredIN\!\!\! & Places & Plantae & Cars \\ \midrule
%     -             & 49.34{\scriptsize$\pm$.77} & 48.96{\scriptsize$\pm$.86} & 46.24{\scriptsize$\pm$.78} & 33.08{\scriptsize$\pm$.59} & 29.55{\scriptsize$\pm$.52} \\
%     $+$ HFlip     & 49.58{\scriptsize$\pm$.76} & 49.46{\scriptsize$\pm$.86} & 46.50{\scriptsize$\pm$.76} & 33.22{\scriptsize$\pm$.59} & 29.67{\scriptsize$\pm$.50} \\
%     $+$ RCrop & 51.24{\scriptsize$\pm$.80} & 48.29{\scriptsize$\pm$.86} & 46.63{\scriptsize$\pm$.80} & 34.41{\scriptsize$\pm$.62} & 29.91{\scriptsize$\pm$.56}\\
%     $+$ CJitter   & 49.29{\scriptsize$\pm$.76} & 48.61{\scriptsize$\pm$.84} & 46.27{\scriptsize$\pm$.75} & 33.29{\scriptsize$\pm$.59} & 29.50{\scriptsize$\pm$.51} \\
%     $+$ Base Aug   & 51.59{\scriptsize$\pm$.79} & 49.01{\scriptsize$\pm$.86} & 47.31{\scriptsize$\pm$.81} & 34.74{\scriptsize$\pm$.61} & 30.12{\scriptsize$\pm$.56} \\
%     $+$ MixUp     & 46.30{\scriptsize$\pm$.73} & 45.81{\scriptsize$\pm$.82} & 43.80{\scriptsize$\pm$.79} & 31.98{\scriptsize$\pm$.56} & 28.97{\scriptsize$\pm$.50} \\
%     $+$ CutMix    & 48.98{\scriptsize$\pm$.77} & 47.93{\scriptsize$\pm$.85} & 46.44{\scriptsize$\pm$.74} & 32.81{\scriptsize$\pm$.57} & 29.16{\scriptsize$\pm$.49} \\ \midrule
%     Aug. & CUB & CropDiseases & EuroSAT & ISIC & ChestX \\ \midrule
%     -             & 37.57{\scriptsize$\pm$.70} & 66.82{\scriptsize$\pm$.89} & 57.25{\scriptsize$\pm$.83} & 31.20{\scriptsize$\pm$.55} & 22.06{\scriptsize$\pm$.38} \\
%     $+$ HFlip     & 38.03{\scriptsize$\pm$.70} & 68.78{\scriptsize$\pm$.90} & 59.35{\scriptsize$\pm$.84} & 31.84{\scriptsize$\pm$.56} & 22.19{\scriptsize$\pm$.36} \\
%     $+$ RCrop & 38.79{\scriptsize$\pm$.73} & 63.52{\scriptsize$\pm$.93} & 56.88{\scriptsize$\pm$.84} & 32.14{\scriptsize$\pm$.57} & 21.77{\scriptsize$\pm$.38} \\
%     $+$ CJitter   & 37.67{\scriptsize$\pm$.70} & 67.28{\scriptsize$\pm$.90} & 58.12{\scriptsize$\pm$.86} & 31.69{\scriptsize$\pm$.54} & 21.94{\scriptsize$\pm$.38} \\
%     $+$ Base Aug   & 39.57{\scriptsize$\pm$.73} & 65.49{\scriptsize$\pm$.91} & 58.30{\scriptsize$\pm$.86} & 32.97{\scriptsize$\pm$.56} & 22.07{\scriptsize$\pm$.37} \\
%     $+$ MixUp     & 35.89{\scriptsize$\pm$.69} & 63.67{\scriptsize$\pm$.88} & 50.53{\scriptsize$\pm$.87} & 31.22{\scriptsize$\pm$.54} & 22.15{\scriptsize$\pm$.37} \\
%     $+$ CutMix    & 37.15{\scriptsize$\pm$.70} & 67.38{\scriptsize$\pm$.91} & 59.61{\scriptsize$\pm$.86} & 31.34{\scriptsize$\pm$.56} & 21.81{\scriptsize$\pm$.39} \\  \midrule
%     \multicolumn{6}{l}{$k$ = 5} \\ \midrule
%     Aug. & miniIN & tieredIN & Places & Plantae & Cars \\ \midrule
%     -             & 75.55{\scriptsize$\pm$.60} & 73.59{\scriptsize$\pm$.74} & 70.60{\scriptsize$\pm$.68} & 53.45{\scriptsize$\pm$.74} & {49.85}{\scriptsize$\pm$.73} \\
%     $+$ HFlip     & 76.17{\scriptsize$\pm$.59} & 74.79{\scriptsize$\pm$.73} & 72.19{\scriptsize$\pm$.67} & 53.04{\scriptsize$\pm$.72} & 48.53{\scriptsize$\pm$.72} \\
%     $+$ RCrop     & 74.56{\scriptsize$\pm$.63} & 71.72{\scriptsize$\pm$.72} & 69.10{\scriptsize$\pm$.68} & 55.26{\scriptsize$\pm$.73} & 49.39{\scriptsize$\pm$.73} \\
%     $+$ CJitter   & 75.71{\scriptsize$\pm$.60} & 73.51{\scriptsize$\pm$.74} & 70.83{\scriptsize$\pm$.68} & 53.91{\scriptsize$\pm$.75} & 50.32{\scriptsize$\pm$.71} \\
%     $+$ Base Aug     & 74.74{\scriptsize$\pm$.62} & 72.25{\scriptsize$\pm$.74} & 69.79{\scriptsize$\pm$.68} & 56.10{\scriptsize$\pm$.71} & 51.15{\scriptsize$\pm$.73}\\
%     $+$ MixUp     & 71.72{\scriptsize$\pm$.65} & 70.66{\scriptsize$\pm$.76} & 66.53{\scriptsize$\pm$.73} & 52.11{\scriptsize$\pm$.75} & 47.89{\scriptsize$\pm$.68} \\
%     $+$ CutMix    & 74.04{\scriptsize$\pm$.63} & 72.32{\scriptsize$\pm$.75} & 69.98{\scriptsize$\pm$.71} & 52.47{\scriptsize$\pm$.72} & 48.30{\scriptsize$\pm$.70} \\ \midrule
%     Aug. & CUB & CropDiseases & EuroSAT & ISIC & ChestX \\ \midrule
%     -             & {59.93}{\scriptsize$\pm$.79} & {91.64}{\scriptsize$\pm$.49} & 82.32{\scriptsize$\pm$.57} & {48.82}{\scriptsize$\pm$.62} & 25.97{\scriptsize$\pm$.40} \\
%     $+$ HFlip     & 58.05{\scriptsize$\pm$.78} & 92.70{\scriptsize$\pm$.46} & 83.52{\scriptsize$\pm$.56} & 50.24{\scriptsize$\pm$.61} & 26.05{\scriptsize$\pm$.43} \\
%     $+$ RCrop    & 60.44{\scriptsize$\pm$.76} & 90.91{\scriptsize$\pm$.48} & 78.97{\scriptsize$\pm$.62} & 48.37{\scriptsize$\pm$.56} & 27.28{\scriptsize$\pm$.42} \\
%     $+$ CJitter   & 60.12{\scriptsize$\pm$.78} & 91.84{\scriptsize$\pm$.49} & 81.98{\scriptsize$\pm$.59} & 48.43{\scriptsize$\pm$.60} & 26.14{\scriptsize$\pm$.43} \\
%     $+$ Base Aug & 62.43{\scriptsize$\pm$.74} & 91.54{\scriptsize$\pm$.46} & 79.71{\scriptsize$\pm$.61} & 48.42{\scriptsize$\pm$.59} & 27.93{\scriptsize$\pm$.43} \\
%     $+$ MixUp     & 58.16{\scriptsize$\pm$.76} & 90.12{\scriptsize$\pm$.52} & 75.23{\scriptsize$\pm$.66} & 48.65{\scriptsize$\pm$.61} & 25.90{\scriptsize$\pm$.42} \\
%     $+$ CutMix    & 56.84{\scriptsize$\pm$.78} & 91.84{\scriptsize$\pm$.49} & 82.93{\scriptsize$\pm$.56} & 46.39{\scriptsize$\pm$.60} & 25.90{\scriptsize$\pm$.42} \\ \midrule
%     \multicolumn{6}{l}{$k$ = 20} \\ \midrule
%     Aug. & miniIN & \!\!\!\!tieredIN\!\!\!\! & Places & Plantae & Cars \\ \midrule
%     -             & 86.94{\scriptsize$\pm$.44} & 84.48{\scriptsize$\pm$.59} & 81.30{\scriptsize$\pm$.53} & 69.08{\scriptsize$\pm$.68} & 70.62{\scriptsize$\pm$.64} \\
%     $+$ HFlip     & 87.23{\scriptsize$\pm$.44} & 85.06{\scriptsize$\pm$.56} & 81.73{\scriptsize$\pm$.54} & 70.02{\scriptsize$\pm$.69} & 73.14{\scriptsize$\pm$.63} \\
%     $+$ RCrop     & 85.40{\scriptsize$\pm$.47} & 83.40{\scriptsize$\pm$.57} & 80.59{\scriptsize$\pm$.54} & 70.78{\scriptsize$\pm$.66} & 69.63{\scriptsize$\pm$.61} \\
%     $+$ CJitter   & 87.00{\scriptsize$\pm$.44} & 84.63{\scriptsize$\pm$.58} & 81.35{\scriptsize$\pm$.53} & 69.41{\scriptsize$\pm$.68} & 71.49{\scriptsize$\pm$.63} \\
%     $+$ Base Aug & 85.83{\scriptsize$\pm$.47} & 83.87{\scriptsize$\pm$.57} & 81.15{\scriptsize$\pm$.53} & 71.51{\scriptsize$\pm$.65} & 71.46{\scriptsize$\pm$.59} \\
%     $+$ MixUp     & 84.26{\scriptsize$\pm$.48} & 82.65{\scriptsize$\pm$.58} & 78.52{\scriptsize$\pm$.57} & 67.78{\scriptsize$\pm$.69} & 69.55{\scriptsize$\pm$.64} \\
%     $+$ CutMix    & 85.58{\scriptsize$\pm$.46} & 83.35{\scriptsize$\pm$.59} & 80.69{\scriptsize$\pm$.54} & 68.10{\scriptsize$\pm$.65} & 69.02{\scriptsize$\pm$.63} \\ \midrule
%     Aug. & CUB & \!\!\!\!CropDiseases\!\!\!\! & EuroSAT & ISIC & ChestX \\ \midrule
%     -             & 75.91{\scriptsize$\pm$.67} & 97.72{\scriptsize$\pm$.22} & 92.54{\scriptsize$\pm$.36} & 62.36{\scriptsize$\pm$.59} & 32.65{\scriptsize$\pm$.47} \\
%     $+$ HFlip     & 77.39{\scriptsize$\pm$.64} & 98.02{\scriptsize$\pm$.20} & 93.19{\scriptsize$\pm$.33} & 63.62{\scriptsize$\pm$.59} & 32.62{\scriptsize$\pm$.46} \\
%     $+$ RCrop     & 76.26{\scriptsize$\pm$.62} & 97.34{\scriptsize$\pm$.22} & 90.82{\scriptsize$\pm$.39} & 60.97{\scriptsize$\pm$.58} & 33.87{\scriptsize$\pm$.46} \\
%     $+$ CJitter   & 76.54{\scriptsize$\pm$.65} & 97.68{\scriptsize$\pm$.22} & 92.59{\scriptsize$\pm$.35} & 60.66{\scriptsize$\pm$.62} & 33.36{\scriptsize$\pm$.46} \\
%     $+$ Base Aug & 77.78{\scriptsize$\pm$.60} & 97.53{\scriptsize$\pm$.22} & 91.71{\scriptsize$\pm$.35} & 60.50{\scriptsize$\pm$.57} & 34.05{\scriptsize$\pm$.44} \\
%     $+$ MixUp     & 75.59{\scriptsize$\pm$.68} & 96.77{\scriptsize$\pm$.27} & 88.86{\scriptsize$\pm$.43} & 62.27{\scriptsize$\pm$.56} & 32.02{\scriptsize$\pm$.45} \\
%     $+$ CutMix    & 72.33{\scriptsize$\pm$.67} & 97.52{\scriptsize$\pm$.23} & 92.26{\scriptsize$\pm$.35} & 59.54{\scriptsize$\pm$.56} & 32.20{\scriptsize$\pm$.46} \\ 
%      \bottomrule
%     \end{tabular}}
%     \caption{5-way $k$-shot performance according to data augmentation techniques. The pre-trained ResNet10 on miniIN is fine-tuned.}\label{tab:miniIN_1_shot_da}
% \end{table}




% \begin{figure}[t]
%     \centering
%     \begin{subfigure}[h]{0.325\linewidth}
%     \includegraphics[width=\linewidth]{figure/interpolation/LPFT_interpolation_mini_test_1.pdf}
%         \caption{miniIN ($k=1$)}
%     \end{subfigure}
%     \begin{subfigure}[h]{0.325\linewidth}
%     \includegraphics[width=\linewidth]{figure/interpolation/LPFT_interpolation_mini_test_5.pdf}
%         \caption{miniIN ($k=5$)}
%     \end{subfigure}
%     \begin{subfigure}[h]{0.325\linewidth}
%     \includegraphics[width=\linewidth]{figure/interpolation/LPFT_interpolation_mini_test_20.pdf}
%         \caption{miniIN ($k=20$)}
%     \end{subfigure}
    
%     \begin{subfigure}[h]{0.325\linewidth}
%     \includegraphics[width=\linewidth]{figure/interpolation/LPFT_interpolation_cub_1.pdf}
%         \caption{CUB ($k=1$)}
%     \end{subfigure}
%     \begin{subfigure}[h]{0.325\linewidth}
%     \includegraphics[width=\linewidth]{figure/interpolation/LPFT_interpolation_cub_5.pdf}
%         \caption{CUB ($k=5$)}
%     \end{subfigure}
%     \begin{subfigure}[h]{0.325\linewidth}
%     \includegraphics[width=\linewidth]{figure/interpolation/LPFT_interpolation_cub_20.pdf}
%         \caption{CUB ($k=20$)}
%     \end{subfigure}
%     \caption{5-way $k$-shot performance according to the updated layers. ResNet consists of a stem convolution layer (stem), four stages (s1-s4), and a classifier. LS updates only a classifier, where FT updates the entire model.}
%     \label{fig:layer_abla}
% \end{figure}





% % \clearpage
% \newpage
% \section{V-measure of with and without MixUp on Other Datasets}\label{appx:v_measure_other_mixup}
% We analyze FT with and without MixUp by comparing V-measure of FT and LP on $k \in \{1,5,10,20\}$.
% The trend is the opposite of Section \ref{sec:analysis1} and Appendix \ref{appx:v_measure_other}. Even though the number of shots increases from $k$=1 to $k$=20, many dots indicating a change in V-measure of each episode are placed under $y=x$ line, and more of them are colored blue. This means that MixUp rather deteriorates the effectiveness of more shots, degrading the ability of the updated feature extractor by learning augmented images. 

% % \begin{figure}[h!]
% % \centering
% %      \begin{subfigure}[h]{0.255\linewidth}
% %          \includegraphics[width=\linewidth]{figure/v_score/mixup/1shot_mini_test_mixup.pdf}
% %      \end{subfigure}
% %      \begin{subfigure}[h]{0.22\linewidth}
% %          \includegraphics[width=\linewidth]{figure/v_score/mixup/5shot_mini_test_mixup.pdf}
% %      \end{subfigure}
% %      \begin{subfigure}[h]{0.22\linewidth}
% %          \includegraphics[width=\linewidth]{figure/v_score/mixup/10shot_mini_test_mixup.pdf}
% %      \end{subfigure}
% %      \begin{subfigure}[h]{0.22\linewidth}
% %          \includegraphics[width=\linewidth]{figure/v_score/mixup/20shot_mini_test_mixup.pdf}
% %      \end{subfigure}
     
     
% %      \begin{subfigure}[h]{0.255\linewidth}
% %          \includegraphics[width=\linewidth]{figure/v_score/mixup/1shot_tiered_test_mixup.pdf}
% %      \end{subfigure}
% %      \begin{subfigure}[h]{0.22\linewidth}
% %          \includegraphics[width=\linewidth]{figure/v_score/mixup/5shot_tiered_test_mixup.pdf}
% %      \end{subfigure}
% %      \begin{subfigure}[h]{0.22\linewidth}
% %          \includegraphics[width=\linewidth]{figure/v_score/mixup/10shot_tiered_test_mixup.pdf}
% %      \end{subfigure}
% %      \begin{subfigure}[h]{0.22\linewidth}
% %          \includegraphics[width=\linewidth]{figure/v_score/mixup/20shot_tiered_test_mixup.pdf}
% %      \end{subfigure}
     
% %      \begin{subfigure}[h]{0.255\linewidth}
% %          \includegraphics[width=\linewidth]{figure/v_score/mixup/1shot_places_mixup.pdf}
% %      \end{subfigure}
% %      \begin{subfigure}[h]{0.22\linewidth}
% %          \includegraphics[width=\linewidth]{figure/v_score/mixup/5shot_places_mixup.pdf}
% %      \end{subfigure}
% %      \begin{subfigure}[h]{0.22\linewidth}
% %          \includegraphics[width=\linewidth]{figure/v_score/mixup/10shot_places_mixup.pdf}
% %      \end{subfigure}
% %      \begin{subfigure}[h]{0.22\linewidth}
% %          \includegraphics[width=\linewidth]{figure/v_score/mixup/20shot_places_mixup.pdf}
% %      \end{subfigure}
     
% %      \begin{subfigure}[h]{0.255\linewidth}
% %          \includegraphics[width=\linewidth]{figure/v_score/mixup/1shot_plantae_mixup.pdf}
% %      \end{subfigure}
% %      \begin{subfigure}[h]{0.22\linewidth}
% %          \includegraphics[width=\linewidth]{figure/v_score/mixup/5shot_plantae_mixup.pdf}
% %      \end{subfigure}
% %      \begin{subfigure}[h]{0.22\linewidth}
% %          \includegraphics[width=\linewidth]{figure/v_score/mixup/10shot_plantae_mixup.pdf}
% %      \end{subfigure}
% %      \begin{subfigure}[h]{0.22\linewidth}
% %          \includegraphics[width=\linewidth]{figure/v_score/mixup/20shot_plantae_mixup.pdf}
% %      \end{subfigure}
     
% %      \begin{subfigure}[h]{0.255\linewidth}
% %          \includegraphics[width=\linewidth]{figure/v_score/mixup/1shot_cars_mixup.pdf}
% %      \end{subfigure}
% %      \begin{subfigure}[h]{0.22\linewidth}
% %          \includegraphics[width=\linewidth]{figure/v_score/mixup/5shot_cars_mixup.pdf}
% %      \end{subfigure}
% %      \begin{subfigure}[h]{0.22\linewidth}
% %          \includegraphics[width=\linewidth]{figure/v_score/mixup/10shot_cars_mixup.pdf}
% %      \end{subfigure}
% %      \begin{subfigure}[h]{0.22\linewidth}
% %          \includegraphics[width=\linewidth]{figure/v_score/mixup/20shot_cars_mixup.pdf}
% %      \end{subfigure}
     
% %      \begin{subfigure}[h]{0.255\linewidth}
% %          \includegraphics[width=\linewidth]{figure/v_score/mixup/1shot_cub_mixup.pdf}
% %      \end{subfigure}
% %      \begin{subfigure}[h]{0.22\linewidth}
% %          \includegraphics[width=\linewidth]{figure/v_score/mixup/5shot_cub_mixup.pdf}
% %      \end{subfigure}
% %      \begin{subfigure}[h]{0.22\linewidth}
% %          \includegraphics[width=\linewidth]{figure/v_score/mixup/10shot_cub_mixup.pdf}
% %      \end{subfigure}
% %      \begin{subfigure}[h]{0.22\linewidth}
% %          \includegraphics[width=\linewidth]{figure/v_score/mixup/20shot_cub_mixup.pdf}
% %      \end{subfigure}
     
% %      \begin{subfigure}[h]{0.255\linewidth}
% %          \includegraphics[width=\linewidth]{figure/v_score/mixup/1shot_crop_mixup.pdf}
% %      \end{subfigure}
% %      \begin{subfigure}[h]{0.22\linewidth}
% %          \includegraphics[width=\linewidth]{figure/v_score/mixup/5shot_crop_mixup.pdf}
% %      \end{subfigure}
% %      \begin{subfigure}[h]{0.22\linewidth}
% %          \includegraphics[width=\linewidth]{figure/v_score/mixup/10shot_crop_mixup.pdf}
% %      \end{subfigure}
% %      \begin{subfigure}[h]{0.22\linewidth}
% %          \includegraphics[width=\linewidth]{figure/v_score/mixup/20shot_crop_mixup.pdf}
% %      \end{subfigure}
     
% %      \begin{subfigure}[h]{0.255\linewidth}
% %          \includegraphics[width=\linewidth]{figure/v_score/mixup/1shot_euro_mixup.pdf}
% %      \end{subfigure}
% %      \begin{subfigure}[h]{0.22\linewidth}
% %          \includegraphics[width=\linewidth]{figure/v_score/mixup/5shot_euro_mixup.pdf}
% %      \end{subfigure}
% %      \begin{subfigure}[h]{0.22\linewidth}
% %          \includegraphics[width=\linewidth]{figure/v_score/mixup/10shot_euro_mixup.pdf}
% %      \end{subfigure}
% %      \begin{subfigure}[h]{0.22\linewidth}
% %          \includegraphics[width=\linewidth]{figure/v_score/mixup/20shot_euro_mixup.pdf}
% %      \end{subfigure}
     
% %      \begin{subfigure}[h]{0.255\linewidth}
% %          \includegraphics[width=\linewidth]{figure/v_score/mixup/1shot_isic_mixup.pdf}
% %      \end{subfigure}
% %      \begin{subfigure}[h]{0.22\linewidth}
% %          \includegraphics[width=\linewidth]{figure/v_score/mixup/5shot_isic_mixup.pdf}
% %      \end{subfigure}
% %      \begin{subfigure}[h]{0.22\linewidth}
% %          \includegraphics[width=\linewidth]{figure/v_score/mixup/10shot_isic_mixup.pdf}
% %      \end{subfigure}
% %      \begin{subfigure}[h]{0.22\linewidth}
% %          \includegraphics[width=\linewidth]{figure/v_score/mixup/20shot_isic_mixup.pdf}
% %      \end{subfigure}
     
     
% %      \begin{subfigure}[h]{0.255\linewidth}
% %          \includegraphics[width=\linewidth]{figure/v_score/mixup/1shot_chest_mixup.pdf}
% %      \end{subfigure}
% %      \begin{subfigure}[h]{0.22\linewidth}
% %          \includegraphics[width=\linewidth]{figure/v_score/mixup/5shot_chest_mixup.pdf}
% %      \end{subfigure}
% %      \begin{subfigure}[h]{0.22\linewidth}
% %          \includegraphics[width=\linewidth]{figure/v_score/mixup/10shot_chest_mixup.pdf}
% %      \end{subfigure}
% %      \begin{subfigure}[h]{0.22\linewidth}
% %          \includegraphics[width=\linewidth]{figure/v_score/mixup/20shot_chest_mixup.pdf}
% %      \end{subfigure}
% %      \caption{Feature extractor’s clustering ability by V-measure and performance differences between LP and FT. The pre-trained model is ResNet10 on miniIN.} \label{fig:v_measure_mixup}
% % \end{figure}

% % 4. DA for CDFSL
% %\newpage
% \section{Performance of LP with Data Augmentation}\label{appx:DA_LP}

% We provide extended results on performance of LP with data augmentation. Table \ref{fig:DA_LP} shows how performance changes when different basic image manipulation methods are applied in LP. This experiment is conducted for $k$=1 and $k$=5 on BSCD-FSL datasets, using ResNet10 pre-trained on miniIN. Unlike the general wisdom that data augmentation improves performance, the performance of LP with data augmentation drops significantly. The result shows that basic image manipulation methods rather negatively affect the ability of the classifier, and this effect is larger in $1$-shot setting, where the performance degrades more than $5$-shot. This demonstrates that the linear classifier trained with fewer samples is more sensitive to image transformations. 


% % \begin{table*}[h]
% % \vskip 0.10in
% % \centering
% % \footnotesize
% % \begin{tabular}{cc|ccccc}
% %     \toprule
% %          {} & {Base} & {ResizedCrop} & {ColoredJitter} & {HorizontalFlip} & {GrayScale} & {GaussianBlur}\\
% %     \midrule
% %     {miniImageNet test} & 77.95{\scriptsize$\pm$.61} & 75.08{\scriptsize$\pm$.63} & 76.45{\scriptsize$\pm$.66} & 74.89{\scriptsize$\pm$.64} & 77.95{\scriptsize$\pm$.62} & 77.94{\scriptsize$\pm$.61}\\
% %     \midrule
% %     {CropDisease} & 91.50{\scriptsize$\pm$.49} & 87.55{\scriptsize$\pm$.56} & {89.21}{\scriptsize$\pm$.56} & 90.64{\scriptsize$\pm$.52} & 91.22{\scriptsize$\pm$.50} & 91.39{\scriptsize$\pm$.50} \\
% %     \midrule
% %     {EuroSAT} & 84.08{\scriptsize$\pm$.60} & 79.48{\scriptsize$\pm$.61} & 59.70{\scriptsize$\pm$.90} & 82.09{\scriptsize$\pm$.59} & 84.26{\scriptsize$\pm$.60} & 84.02{\scriptsize$\pm$.60} \\
% %     \midrule
% %     {ISIC} & 40.39{\scriptsize$\pm$.55} & 44.55{\scriptsize$\pm$.58} & 40.56{\scriptsize$\pm$.56} & 44.94{\scriptsize$\pm$.60} & 40.29{\scriptsize$\pm$.55} & 40.44{\scriptsize$\pm$.56} \\
% %     \midrule
% %     {ChestX} & 26.75{\scriptsize$\pm$.43} & 25.62{\scriptsize$\pm$.41} & 26.89{\scriptsize$\pm$.43} & 25.94{\scriptsize$\pm$.40} & 26.78{\scriptsize$\pm$.43} & 26.78{\scriptsize$\pm$.42}\\
% %     \bottomrule
% % \end{tabular}
% % \caption{5-way 5-shot performance according to augmentation methods}
% % \end{table*}

% % 1shot
%     % {miniImageNet test} & 56.47{\scriptsize$\pm$.80} & 50.48{\scriptsize$\pm$.81} & 56.10{\scriptsize$\pm$.81} & 48.06{\scriptsize$\pm$.84} & 56.45{\scriptsize$\pm$.82} & 57.21{\scriptsize$\pm$.84}  \\
%     % \midrule
%     % {CropDisease} & 73.12{\scriptsize$\pm$.88} & 59.08{\scriptsize$\pm$.97} & 59.28{\scriptsize$\pm$.94} & 62.39{\scriptsize$\pm$.96} & 72.10{\scriptsize$\pm$.88} & 47.69{\scriptsize$\pm$1.10}\\
%     % \midrule
%     % {EuroSAT} & 64.72{\scriptsize$\pm$.88} & 55.08{\scriptsize$\pm$.86} & 64.87{\scriptsize$\pm$.88} & 56.03{\scriptsize$\pm$.84} & 64.94{\scriptsize$\pm$.86} & 46.26{\scriptsize$\pm$.78}\\
%     % \midrule
%     % {ISIC} & 29.39{\scriptsize$\pm$.53} & 30.56{\scriptsize$\pm$.53} & 29.47{\scriptsize$\pm$.56} & 29.61{\scriptsize$\pm$.51} & 29.42{\scriptsize$\pm$.5} & 25.94{\scriptsize$\pm$.47} \\
%     % \midrule
%     % {ChestX} & 21.45{\scriptsize$\pm$.31} & 21.90{\scriptsize$\pm$.30} & 22.85{\scriptsize$\pm$.41} & 21.78{\scriptsize$\pm$.35} & 22.67{\scriptsize$\pm$.41} & 21.30{\scriptsize$\pm$.29}\\
%     % \bottomrule





% % 5. Related Works
% % \section{Additional Related Works}\label{appx:related}
% % \textbf{Few-Shot Learning (FSL)} focuses on underlying problems of deep learning where there are few training samples available. 
% % % 
% % There are two dominant approaches for FSL, meta-learning-based and transfer learning-based. To predict class, the former uses prior knowledge which is generalized across tasks, while the latter uses transferred knowledge learned from large source data. 
% % % 
% % Meta-learning aims to design a generalized model that adapts to new tasks quickly, by learning a good initialization\,\citep{finn2017model, li2017meta, lee2018gradient, rajeswaran2019meta, oh2021boil}, learning the metrics\,\citep{koch2015siamese, vinyals2016matching, snell2017prototypical, sung2018learning}, or learning generative models to augment few-shot data\,\citep{antoniou2017data, hariharan2017low}.
% % %
% % In contrast, transfer learning aims to transfer knowledge from source tasks to few-shot tasks.
% % %
% % By the capacity of deep backbones learned on ImageNet\,\citep{deng2009imagenet}, pre-trained knowledge is effectively transferred to different target datasets and target tasks\,\citep{luo2017label, azadi2018multi, liu2018feature, chen2019closer, dhillon2019baseline, luo2021rectifying}.

% % For more realistic FSL, cross-domain few-shot learning (CD-FSL), where there is a large distributional shift from source to target domain, has gained increased attention. 
% % %
% % \citet{guo2020broader} provided CD-FSL benchmark and demonstrated that transfer-based models achieved higher performances than existing meta-learning approaches. 
% % % 
% % Therefore, to address a distribution shift challenge, prior works have focused on transfer-learning based approaches by utilizing semi-supervised methods\,\citep{phoo2020self,islam2021dynamic} or unsupervised methods\,\citet{luo2017label, phoo2020self, das2021confess}.


% % \textbf{Data Augmentation (DA)} is a general technique to prevent overfitting on training distribution and increase generalization performance\,\citep{simard2003best, krizhevsky2012imagenet}.
% % %
% % % Augmentation techniques can be divided into three main categories: basic image manipulation, data-mixing, and deep learning approach\,\citep{shorten2019survey}.
% % %
% % Basic image manipulation methods such as flipping, rotating, and cropping are the most generic and prevalent practice in computer vision tasks.
% % %
% %  Data-mixing methods include MixUp \citep{zhang2017mixup}, CutMix \citep{yun2019cutmix}, and PuzzleMix \citep{kim2020puzzle}, which mix two images while mixing corresponding class labels.
% % %
% % %Meanwhile, \citet{verma2019manifold} proposed a manifold mixup which mixes feature representation of two different images in manifold space. 
% % In addition, there are deep learning approaches for data augmentation. These approaches include generating images which are similar\,\citep{mirza2014conditional}, style-transferred\,\citep{gatys2016image} and domain-transferred\,\citep{zhu2017unpaired}.
% % %
% % In our study, we focus on basic image manipulations and data-mixing methods because there is no sufficient data to train generative models during fine-tuning.

% %\newpage

% \subsection{Body Updates with Augmentation}
% \begin{table}[h]
%     %\vskip 0.10in
%     \centering
%     \resizebox{\linewidth}{!}{
%     %\footnotesize\addtolength{\tabcolsep}{-2.4pt}
%     \begin{tabular}{cccccc}
%     \toprule
%      Method & miniIN & tieredIN & Places & Plantae & Cars\\ \midrule
%      \textbf{FT} & 75.55{\scriptsize$\pm$.60} & 73.59{\scriptsize$\pm$.74} & 70.60{\scriptsize$\pm$.68} & 53.45{\scriptsize$\pm$.74} & 49.85{\scriptsize$\pm$.73}\\
%      Body & {70.47}{\scriptsize$\pm$.72} & {67.72}{\scriptsize$\pm$.77} & {66.39}{\scriptsize$\pm$.73} & {51.99}{\scriptsize$\pm$.72} & 48.87{\scriptsize$\pm$.68}\\
%      Body+RCrop & 70.77{\scriptsize$\pm$.69} & 68.06{\scriptsize$\pm$.75} & 66.87{\scriptsize$\pm$.72} & 52.29{\scriptsize$\pm$.73} & 48.71{\scriptsize$\pm$.69} \\
%      Body+MixUp & 68.31\scriptsize{\scriptsize$\pm$.71} & 66.32\scriptsize{\scriptsize$\pm$.81} & 64.47\scriptsize{\scriptsize$\pm$.75} & 50.82{\scriptsize$\pm$.75}& 47.43{\scriptsize$\pm$.71} \\
%      \midrule
%      Method & CUB & \!\!\!\!CropDiseases\!\!\!\! & EuroSAT & ISIC & ChestX \\ \midrule
%      \textbf{FT} & 59.93{\scriptsize$\pm$.79} & 91.64{\scriptsize$\pm$.49} & 82.32{\scriptsize$\pm$.57} & 48.82{\scriptsize$\pm$.62} & 25.97{\scriptsize$\pm$.40} \\
%      Body & 56.53{\scriptsize$\pm$.78} & 91.48{\scriptsize$\pm$.53} & {82.08}{\scriptsize$\pm$.62} & 47.35{\scriptsize$\pm$.60} & {26.07}{\scriptsize$\pm$.42} \\
%      Body+RCrop & 56.76{\scriptsize$\pm$.78} & 92.03{\scriptsize$\pm$.48} & 81.88{\scriptsize$\pm$.63} & 47.10{\scriptsize$\pm$.63} & 26.36{\scriptsize$\pm$.43} \\
%      Body+MixUp & 55.00{\scriptsize$\pm$.79} & 90.44{\scriptsize$\pm$.56} & 78.36{\scriptsize$\pm$.66} & 47.96{\scriptsize$\pm$.62} & {26.09}{\scriptsize$\pm$.43} \\
%      \bottomrule
%     \end{tabular}}
%     \caption{5-way 5-shot performance of Body updates with fixed random classifier. The backbone is ResNet10 pre-trained on miniIN.}\label{tab:body_update}
% \end{table}

% \subsection{Base Augmentation with Label Smoothing}
% \begin{table}[h]
%     %\vskip 0.10in
%     \centering
%     \resizebox{\linewidth}{!}{
%     %\footnotesize\addtolength{\tabcolsep}{-3.2pt}
%     \begin{tabular}{cccccccccccc}
%     \toprule
%     $k$ & Update & miniIN & tieredIN & Places & Plantae & Cars\\ \midrule
%     \multirow{3}{*}{1} & {-} & 49.57{\scriptsize$\pm$.79} & 49.10{\scriptsize$\pm$.90} & 45.44{\scriptsize$\pm$.79} & 33.35{\scriptsize$\pm$.59} & {29.49}{\scriptsize$\pm$.54}\\ 
%      & {+ Base} & 52.02{\scriptsize$\pm$.79} & 49.12{\scriptsize$\pm$.89} & 46.75{\scriptsize$\pm$.80} & 34.93{\scriptsize$\pm$.62} & 30.38{\scriptsize$\pm$.55}\\
%      & {Base + ls} & 49.91{\scriptsize$\pm$.78} & 47.48{\scriptsize$\pm$.84} & 45.54{\scriptsize$\pm$.78} & 34.29{\scriptsize$\pm$.64} & 30.14 {\scriptsize$\pm$.57}\\
%     \midrule
%     \multirow{3}{*}{5} & {-} & 75.67{\scriptsize$\pm$.65} & 73.60{\scriptsize$\pm$.78} & 70.05{\scriptsize$\pm$.71} & 53.19{\scriptsize$\pm$.73} & {49.26}{\scriptsize$\pm$.70}\\ 
%     & {+ Base} & 74.55{\scriptsize$\pm$.65} & 72.16{\scriptsize$\pm$.73} & 69.54{\scriptsize$\pm$.70} & 55.90{\scriptsize$\pm$.76} & 50.88{\scriptsize$\pm$.70}\\
%     & {Base + ls} & 74.23{\scriptsize$\pm$.63} & 71.72{\scriptsize$\pm$.72} & 69.16{\scriptsize$\pm$.70} & 54.99{\scriptsize$\pm$.74} & 49.91{\scriptsize$\pm$.68}\\
%     \midrule
%     $k$ & Update & CUB & CropDiseases & EuroSAT & ISIC & ChestX\\ \midrule
%     \multirow{3}{*}{1} & {-} & 37.54{\scriptsize$\pm$.71} & 66.78{\scriptsize$\pm$.91} & 56.45{\scriptsize$\pm$.84} & {31.03}{\scriptsize$\pm$.55} & 22.35{\scriptsize$\pm$.38} \\ 
%      & {+ Base} & 39.06{\scriptsize$\pm$.75} & 64.84{\scriptsize$\pm$.93} & 56.40{\scriptsize$\pm$.84} & 32.12{\scriptsize$\pm$.59} & 22.06{\scriptsize$\pm$.38}\\
%      & {Base + ls} & 38.59{\scriptsize$\pm$.70} & 64.46{\scriptsize$\pm$.92} & 	56.01{\scriptsize$\pm$.85} & {31.77}{\scriptsize$\pm$.58}  & 22.19{\scriptsize$\pm$.36}\\
%     \midrule
%     \multirow{3}{*}{5} & {-} & {59.35}{\scriptsize$\pm$.80} & {92.14}{\scriptsize$\pm$.49} & 82.58{\scriptsize$\pm$.60} & {48.35}{\scriptsize$\pm$.62} & 26.30{\scriptsize$\pm$.24} \\ 
%     & {+ Base} & 61.61{\scriptsize$\pm$.76} & 90.69{\scriptsize$\pm$.50} & 77.40{\scriptsize$\pm$.63} & 46.96{\scriptsize$\pm$.66} & 26.55{\scriptsize$\pm$.42} \\
%     & {Base + ls} & 60.29{\scriptsize$\pm$.76} & 91.06{\scriptsize$\pm$.48} & 79.94{\scriptsize$\pm$.61} & {47.22}{\scriptsize$\pm$.65}  & 27.51{\scriptsize$\pm$.43}\\
%      \bottomrule
%     \end{tabular}}
%     \caption{5-way $k$-shot performance of base augmentation with label smoothing. The pre-trained ResNet10 on miniIN is fine-tuned.}\label{tab:base_label_smoothing}
% \end{table}

% % \subsection{Manifold MixUp}
% % \begin{table}[h!]
% % %\vskip 0.05in
% % \centering
% % \resizebox{\linewidth}{!}{
% % \begin{tabular}{ccccccc}
% %     \toprule
% %     $k$ & Aug. & miniIN & \!\!\!\!CropDiseases\!\!\!\! & EuroSAT & ISIC & ChestX \\
% %     \midrule
% %     \multirow{4}{*}{1} & -   & 49.57{\scriptsize$\pm$.79} & \!\!\!\!66.78{\scriptsize$\pm$.91}\!\!\!\! & 56.45{\scriptsize$\pm$.84} & 31.03{\scriptsize$\pm$.55} & 22.35{\scriptsize$\pm$.38} \\
% %     & MixUp & 46.50{\scriptsize$\pm$.79} & \!\!\!\!64.62{\scriptsize$\pm$.93}\!\!\!\! & 50.12{\scriptsize$\pm$.78} & 30.42{\scriptsize$\pm$.55} & 22.16{\scriptsize$\pm$.38} \\
% %     & MixUp clean & 47.54{\scriptsize$\pm$.79} & \!\!\!\!65.27{\scriptsize$\pm$.92}\!\!\!\! & 53.03{\scriptsize$\pm$.90} & 30.78{\scriptsize$\pm$.54} & 22.37{\scriptsize$\pm$.38} \\
% %     & Manifold MixUp & 47.84{\scriptsize$\pm$.76} & 65.29{\scriptsize$\pm$.93} & 55.07{\scriptsize$\pm$.83} & 30.43{\scriptsize$\pm$.56} & 22.13{\scriptsize$\pm$.37} \\
% %     & Manifold MixUp clean & 47.82{\scriptsize$\pm$.78} & 64.71{\scriptsize$\pm$.90} & 55.15{\scriptsize$\pm$.81} & 30.31{\scriptsize$\pm$.52} & 22.20{\scriptsize$\pm$.35} \\
% %     \midrule
% %     \multirow{5}{*}{5} & -   & 75.67{\scriptsize$\pm$.65} & \!\!\!\!92.14{\scriptsize$\pm$.49}\!\!\!\! & 82.58{\scriptsize$\pm$.60} & 48.35{\scriptsize$\pm$.62} & 26.30{\scriptsize$\pm$.24} \\
% %     & MixUp & 71.61{\scriptsize$\pm$.67} & \!\!\!\!90.54{\scriptsize$\pm$.54}\!\!\!\! & 75.42{\scriptsize$\pm$.68} & 47.92{\scriptsize$\pm$.62} & 26.08{\scriptsize$\pm$.41} \\
% %     & MixUp clean & 73.48{\scriptsize$\pm$.64} & \!\!\!\!91.03{\scriptsize$\pm$.52}\!\!\!\! & 77.92{\scriptsize$\pm$.63} & 47.53{\scriptsize$\pm$.64} & 26.08{\scriptsize$\pm$.41} \\
% %     & Manifold MixUp   & 74.89{\scriptsize$\pm$.65} & 91.49{\scriptsize$\pm$.52} & 81.58{\scriptsize$\pm$.57} & 47.33{\scriptsize$\pm$.62} & 26.16{\scriptsize$\pm$.42} \\
% %     & Manifold MixUp clean   & 73.93{\scriptsize$\pm$.64} & 90.55{\scriptsize$\pm$.53} & 80.85{\scriptsize$\pm$.61} & 46.60{\scriptsize$\pm$.61} & 25.98{\scriptsize$\pm$.41} \\
% %     %\midrule
% %     % \multirow{4}{*}{20} & -   & 87.38{\scriptsize$\pm$.41} & \!\!\!\!97.89{\scriptsize$\pm$.22}\!\!\!\! & 92.88{\scriptsize$\pm$.35} & 62.98{\scriptsize$\pm$.60} & 32.98{\scriptsize$\pm$.46} \\
% %     % & W+B & 81.34{\scriptsize$\pm$.49} & \!\!\!\!96.32{\scriptsize$\pm$.29}\!\!\!\! & 85.43{\scriptsize$\pm$.50} & 61.33{\scriptsize$\pm$.58} & 31.62{\scriptsize$\pm$.47} \\
% %     % & W   & 85.98{\scriptsize$\pm$.44} & \!\!\!\!97.19{\scriptsize$\pm$.26}\!\!\!\! & 91.65{\scriptsize$\pm$.40} & 62.56{\scriptsize$\pm$.58} & 33.23{\scriptsize$\pm$.48} \\
% %     % & B   & 84.18{\scriptsize$\pm$.46} & \!\!\!\!96.58{\scriptsize$\pm$.29}\!\!\!\! & 87.98{\scriptsize$\pm$.47} & 61.40{\scriptsize$\pm$.61} & 32.07{\scriptsize$\pm$.45} \\
% %     \bottomrule
% % \end{tabular}}
% % \caption{5-way $k$-shot performance according to MixUp strategies} \label{tab:mixup_strat}
% % \end{table}


% % \begin{table}[ht]
% % %\vskip 0.05in
% % \centering
% % \resizebox{\linewidth}{!}{
% % \begin{tabular}{ccccccc}
% %     \toprule
% %     $k$ & MixUp & miniIN & \!\!\!\!CropDiseases\!\!\!\! & EuroSAT & ISIC & ChestX \\
% %     \midrule
% %     \multirow{2}{*}{1} & -   & 49.57{\scriptsize$\pm$.79} & \!\!\!\!66.78{\scriptsize$\pm$.91}\!\!\!\! & 56.45{\scriptsize$\pm$.84} & 31.03{\scriptsize$\pm$.55} & 22.35{\scriptsize$\pm$.38} \\
% %     & B & 47.84{\scriptsize$\pm$.76} & 65.29{\scriptsize$\pm$.93} & 55.07{\scriptsize$\pm$.83} & 30.43{\scriptsize$\pm$.56} & 22.13{\scriptsize$\pm$.37} \\
% %     \midrule
% %     \multirow{4}{*}{5} & -   & 75.67{\scriptsize$\pm$.65} & \!\!\!\!92.14{\scriptsize$\pm$.49}\!\!\!\! & 82.58{\scriptsize$\pm$.60} & 48.35{\scriptsize$\pm$.62} & 26.30{\scriptsize$\pm$.24} \\
% %     & W+B & 74.89{\scriptsize$\pm$.65} & 91.49{\scriptsize$\pm$.52} & 81.58{\scriptsize$\pm$.57} & 47.33{\scriptsize$\pm$.62} & 26.16{\scriptsize$\pm$.42} \\
% %     & W   & 74.68{\scriptsize$\pm$.64} & 91.24{\scriptsize$\pm$.52} & 81.70{\scriptsize$\pm$.61} & 47.69{\scriptsize$\pm$.60} & 26.04{\scriptsize$\pm$.42} \\
% %     & B   & 75.14{\scriptsize$\pm$.63} & 91.80{\scriptsize$\pm$.52} & 81.90{\scriptsize$\pm$.59} & 47.32{\scriptsize$\pm$.62} & 26.26{\scriptsize$\pm$.40} \\
% %     \bottomrule
% % \end{tabular}}
% % \caption{5-way $k$-shot performance according to decomposition of manifold MixUp. W and B indicate manifold MixUp within the same class (for $k>1$) and manifold MixUp between different classes, respectively.}\label{tab:manifold_mixup_decomp}
% % \end{table}

% % \subsection{Multiple Augmentations}
% % \begin{table}[h!]
% % %\vskip 0.05in
% % \centering
% % \resizebox{\linewidth}{!}{
% % \begin{tabular}{ccccccc}
% %     \toprule
% %     $k$ & Aug. & miniIN & \!\!\!\!CropDiseases\!\!\!\! & EuroSAT & ISIC & ChestX \\
% %     \midrule
% %     \multirow{4}{*}{1} & -   & 49.57{\scriptsize$\pm$.79} & \!\!\!\!66.78{\scriptsize$\pm$.91}\!\!\!\! & 56.45{\scriptsize$\pm$.84} & 31.03{\scriptsize$\pm$.55} & 22.35{\scriptsize$\pm$.38} \\
% %     & {$+$ HFlip} & 49.75{\scriptsize$\pm$.80} & 68.48{\scriptsize$\pm$.91} & 58.37{\scriptsize$\pm$.82} & 31.10{\scriptsize$\pm$.57} & 22.30{\scriptsize$\pm$.37} \\
% %     & Manifold MixUp + HFlip  & 48.75{\scriptsize$\pm$.79} & \!\!\!\!67.82{\scriptsize$\pm$.90}\!\!\!\! & 57.78{\scriptsize$\pm$.81} & 30.87{\scriptsize$\pm$.55} & 21.75{\scriptsize$\pm$.38} \\
% %     & CutMix + HFlip & 49.24{\scriptsize$\pm$.78} & \!\!\!\!\textbf{69.80}{\scriptsize$\pm$.86}\!\!\!\! & \textbf{60.45}{\scriptsize$\pm$.84} & 31.00{\scriptsize$\pm$.54} & 22.13{\scriptsize$\pm$.37} \\
% %     % & Manifold MixUp & 47.68{\scriptsize$\pm$.78} & \!\!\!\!64.33{\scriptsize$\pm$.94}\!\!\!\! & 55.12{\scriptsize$\pm$.83} & 30.43{\scriptsize$\pm$.55} & 22.12{\scriptsize$\pm$.37} \\
% %     \midrule
% %     \multirow{4}{*}{5} & -   & 75.67{\scriptsize$\pm$.65} & \!\!\!\!92.14{\scriptsize$\pm$.49}\!\!\!\! & 82.58{\scriptsize$\pm$.60} & 48.35{\scriptsize$\pm$.62} & 26.30{\scriptsize$\pm$.24} \\
% %     & $+$ HFlip     & 76.30{\scriptsize$\pm$.63} & 93.02{\scriptsize$\pm$.47} & 83.62{\scriptsize$\pm$.59} & 49.79{\scriptsize$\pm$.65} & 26.48{\scriptsize$\pm$.40} \\
% %     & Manifold MixUp + HFlip & 75.35{\scriptsize$\pm$.62} & \!\!\!\!92.32{\scriptsize$\pm$.49}\!\!\!\! & 83.00{\scriptsize$\pm$.56} & 48.20{\scriptsize$\pm$.64} & 26.11{\scriptsize$\pm$.43} \\
% %     & CutMix + HFlip & 74.51{\scriptsize$\pm$.64} & \!\!\!\!92.85{\scriptsize$\pm$.46}\!\!\!\! & 83.55{\scriptsize$\pm$.58} & 46.40{\scriptsize$\pm$.58} & 26.59{\scriptsize$\pm$.43} \\
% %     % & Manifold MixUp   & 74.93{\scriptsize$\pm$.64} & \!\!\!\!91.31{\scriptsize$\pm$.52}\!\!\!\! & 81.40{\scriptsize$\pm$.59} & 47.57{\scriptsize$\pm$.61} & 26.26{\scriptsize$\pm$.43} \\
% %     % & Manifold MixUp clean   & 73.85{\scriptsize$\pm$.65} & \!\!\!\!90.52{\scriptsize$\pm$.54}\!\!\!\! & 81.17{\scriptsize$\pm$.59} & 46.50{\scriptsize$\pm$.63} & 25.84{\scriptsize$\pm$.41} \\
% %     \midrule
% %     \multirow{4}{*}{10} & -  & 87.38{\scriptsize$\pm$.41} & \!\!\!\!97.89{\scriptsize$\pm$.22}\!\!\!\! & 92.88{\scriptsize$\pm$.35} & 62.98{\scriptsize$\pm$.60} & 32.98{\scriptsize$\pm$.46} \\
% %     % & +Hflip & 81.34{\scriptsize$\pm$.49} & \!\!\!\!96.32{\scriptsize$\pm$.29}\!\!\!\! & 85.43{\scriptsize$\pm$.50} & 61.33{\scriptsize$\pm$.58} & 31.62{\scriptsize$\pm$.47} \\
% %     & Manifold MixUp + HFlip & 82.52{\scriptsize$\pm$.51} & 96.12{\scriptsize$\pm$.32} & 89.47{\scriptsize$\pm$.42} & 56.30{\scriptsize$\pm$.61} & 29.48{\scriptsize$\pm$.43}\\
% %     & CutMix + HFlip & 81.36{\scriptsize$\pm$.54} & 96.08{\scriptsize$\pm$.33} & 89.24{\scriptsize$\pm$.43} & 53.66{\scriptsize$\pm$.57} & 29.24{\scriptsize$\pm$.43} \\
% %     \bottomrule
% % \end{tabular}}
% % \caption{5-way $k$-shot performance according to Multiple Augmentations} \label{tab:multiple_aug}
% % \end{table}

% % \begin{itemize}
% %     \item clean 실험 문제점 : 데이터가 2배가 됐는데 배치사이즈는 똑같아서 업데이트를 2배함, 배치 내에서 aug -> clean 순으로 데이터가 들어감
% %     \item 왜 image level에서의 mixup과 representation level에서의 mixup이 성능이 일케 다른지? 
% %     \item mixup에 clean data같이 넣어서 학습시킨건 scheduler랑 같은 효과를 주는 것 아닐까! 
% %     \item manifold mixup clean은 왜 떨어지지 근데..? 
% % \end{itemize}


% % \subsection{Self-Supervised Strategies}
% % \begin{table}[h!]
% % %\vskip 0.05in
% % \centering
% % \resizebox{\linewidth}{!}{
% % \begin{tabular}{ccccccc}
% %     \toprule
% %     $k$ & Aug. & miniIN & \!\!\!\!CropDiseases\!\!\!\! & EuroSAT & ISIC & ChestX \\
% %     \midrule
% %     \multirow{5}{*}{1} & -   & 49.57{\scriptsize$\pm$.79} & \!\!\!\!66.78{\scriptsize$\pm$.91}\!\!\!\! & 56.45{\scriptsize$\pm$.84} & 31.03{\scriptsize$\pm$.55} & 22.35{\scriptsize$\pm$.38} \\
% %     & {$+$ SimCLR($\tau$=0.1)} & 49.16{\scriptsize$\pm$.78} & 58.06{\scriptsize$\pm$.106} & 50.49{\scriptsize$\pm$.85} & 30.25{\scriptsize$\pm$.53} & 21.57{\scriptsize$\pm$.34} \\
% %     & {$+$ SimCLR($\tau$=0.3)} & 49.44{\scriptsize$\pm$.84} & 57.85{\scriptsize$\pm$.105} & 51.25{\scriptsize$\pm$.86} & 29.51{\scriptsize$\pm$.50} & 21.53{\scriptsize$\pm$.35} \\
% %     & {$+$ SimCLR($\tau$=0.5)} & 48.86{\scriptsize$\pm$.81} & 56.08{\scriptsize$\pm$.101} & 50.97{\scriptsize$\pm$.86} & 29.39{\scriptsize$\pm$.53} & 21.58{\scriptsize$\pm$.32} \\
% %     & {$+$ SupCon($\tau$=0.5)} & 48.82{\scriptsize$\pm$.81} & 56.74{\scriptsize$\pm$.101} & 51.10{\scriptsize$\pm$.83} & 29.39{\scriptsize$\pm$.52} & 21.33{\scriptsize$\pm$.32} \\
% %     % & CutMix + HFlip & 49.24{\scriptsize$\pm$.78} & \!\!\!\!\textbf{69.80}{\scriptsize$\pm$.86}\!\!\!\! & \textbf{60.45}{\scriptsize$\pm$.84} & 31.00{\scriptsize$\pm$.54} & 22.13{\scriptsize$\pm$.37} \\
% %     % & Manifold MixUp & 47.68{\scriptsize$\pm$.78} & \!\!\!\!64.33{\scriptsize$\pm$.94}\!\!\!\! & 55.12{\scriptsize$\pm$.83} & 30.43{\scriptsize$\pm$.55} & 22.12{\scriptsize$\pm$.37} \\
% %     \midrule
% %     \multirow{2}{*}{5} & -   & 75.67{\scriptsize$\pm$.65} & \!\!\!\!92.14{\scriptsize$\pm$.49}\!\!\!\! & 82.58{\scriptsize$\pm$.60} & 48.35{\scriptsize$\pm$.62} & 26.30{\scriptsize$\pm$.24} \\
% %     % & $+$ HFlip     & 76.30{\scriptsize$\pm$.63} & 93.02{\scriptsize$\pm$.47} & 83.62{\scriptsize$\pm$.59} & 49.79{\scriptsize$\pm$.65} & 26.48{\scriptsize$\pm$.40} \\
% %     & {$+$ SupCon($\tau$=0.5)} & 71.59{\scriptsize$\pm$.66} & 81.11{\scriptsize$\pm$.91} & 73.31{\scriptsize$\pm$.79} & 44.29{\scriptsize$\pm$.64} & 24.35{\scriptsize$\pm$.39} \\
% %     % & CutMix + HFlip & 74.51{\scriptsize$\pm$.64} & \!\!\!\!92.85{\scriptsize$\pm$.46}\!\!\!\! & 83.55{\scriptsize$\pm$.58} & 46.40{\scriptsize$\pm$.58} & 26.59{\scriptsize$\pm$.43} \\
% %     % & Manifold MixUp   & 74.93{\scriptsize$\pm$.64} & \!\!\!\!91.31{\scriptsize$\pm$.52}\!\!\!\! & 81.40{\scriptsize$\pm$.59} & 47.57{\scriptsize$\pm$.61} & 26.26{\scriptsize$\pm$.43} \\
% %     % & Manifold MixUp clean   & 73.85{\scriptsize$\pm$.65} & \!\!\!\!90.52{\scriptsize$\pm$.54}\!\!\!\! & 81.17{\scriptsize$\pm$.59} & 46.50{\scriptsize$\pm$.63} & 25.84{\scriptsize$\pm$.41} \\
% %     % \midrule
% %     % \multirow{4}{*}{20} & -   & 87.38{\scriptsize$\pm$.41} & \!\!\!\!97.89{\scriptsize$\pm$.22}\!\!\!\! & 92.88{\scriptsize$\pm$.35} & 62.98{\scriptsize$\pm$.60} & 32.98{\scriptsize$\pm$.46} \\
% %     % & W+B & 81.34{\scriptsize$\pm$.49} & \!\!\!\!96.32{\scriptsize$\pm$.29}\!\!\!\! & 85.43{\scriptsize$\pm$.50} & 61.33{\scriptsize$\pm$.58} & 31.62{\scriptsize$\pm$.47} \\
% %     % & W   & 85.98{\scriptsize$\pm$.44} & \!\!\!\!97.19{\scriptsize$\pm$.26}\!\!\!\! & 91.65{\scriptsize$\pm$.40} & 62.56{\scriptsize$\pm$.58} & 33.23{\scriptsize$\pm$.48} \\
% %     % & B   & 84.18{\scriptsize$\pm$.46} & \!\!\!\!96.58{\scriptsize$\pm$.29}\!\!\!\! & 87.98{\scriptsize$\pm$.47} & 61.40{\scriptsize$\pm$.61} & 32.07{\scriptsize$\pm$.45} \\
% %     \bottomrule
% % \end{tabular}}
% % \caption{5-way $k$-shot performance according to self-supervised strategies} \label{tab:ssl_loss}
% % \end{table}



% \begin{table}[t]
%     \centering
%     \resizebox{\linewidth}{!}{%
%     \begin{tabular}{ccccccc}
%     \toprule
%     \multicolumn{7}{l}{backbone: ResNet10 pre-trained on miniIN} \\ \midrule
%     $k$ & Update & miniIN & tieredIN & Places & Plantae & Cars \\ \midrule
%     \multirow{2}{*}{1} & LP & \textbf{56.23}{\scriptsize$\pm$.77} & \textbf{55.43}{\scriptsize$\pm$.91} & \textbf{52.83}{\scriptsize$\pm$.81} & \textbf{36.49}{\scriptsize$\pm$.69} & \textbf{29.79}{\scriptsize$\pm$.51} \\
%     & {FT} & 49.34{\scriptsize$\pm$.77} & 48.96{\scriptsize$\pm$.86} & 46.24{\scriptsize$\pm$.78} & 33.08{\scriptsize$\pm$.59} & 29.55{\scriptsize$\pm$.52} \\
%     % & {affinity} & 27.21 & 23.10 & 22.35 & 10.39 & 5.21 \\
%     % & {affinity-sub} & 103.80 & 82.14 & 81.72 & 48.05 & 28.46 \\
%     \midrule
%     \multirow{2}{*}{5} & LP & \textbf{77.77}{\scriptsize$\pm$.61} & \textbf{75.02}{\scriptsize$\pm$.71} & \textbf{73.26}{\scriptsize$\pm$.66} & \textbf{54.21}{\scriptsize$\pm$.74} & 44.92{\scriptsize$\pm$.67} \\
%     & {FT} & 75.55{\scriptsize$\pm$.60} & 73.59{\scriptsize$\pm$.74} & 70.60{\scriptsize$\pm$.68} & 53.45{\scriptsize$\pm$.74} & \textbf{49.85}{\scriptsize$\pm$.73} \\
%     % & affinity & 37.26 & 29.50 & 31.90 & 16.59 & 12.96 \\
%     % & affinity-sub & 98.75 & 69.86 & 83.21 & 48.55 & 46.17 \\
%     % \midrule
%     % \multirow{2}{*}{10} & LP & \textbf{83.06}{\scriptsize$\pm$.52} & {79.80}{\scriptsize$\pm$.68} & \textbf{78.47}{\scriptsize$\pm$.60} & {60.84}{\scriptsize$\pm$.74} & 52.58{\scriptsize$\pm$.69} \\
%     % & {FT} & 82.46{\scriptsize$\pm$.52} & \textbf{80.23}{\scriptsize$\pm$.66} & 76.88{\scriptsize$\pm$.63} & \textbf{61.81}{\scriptsize$\pm$.77} & \textbf{60.07}{\scriptsize$\pm$.69} \\
%     \midrule
%     \multirow{2}{*}{20} & LP & 86.54{\scriptsize$\pm$.44} & 83.26{\scriptsize$\pm$.61} & \textbf{81.53}{\scriptsize$\pm$.53} & 66.52{\scriptsize$\pm$.69} & 60.95{\scriptsize$\pm$.66} \\ 
%      & {FT} & \textbf{86.94}{\scriptsize$\pm$.44} & \textbf{84.48}{\scriptsize$\pm$.59} & 81.30{\scriptsize$\pm$.53} & \textbf{69.08}{\scriptsize$\pm$.68} & \textbf{70.62}{\scriptsize$\pm$.64} \\
%     %  & affinity & 33.66 & 26.25 & 28.04 & 18.09 & 19.83 \\
%     %  & affinity-sub & 68.25 & 49.24 & 55.14 & 40.34 & 50.99 \\
%     \midrule
%     $k$ & Update & CUB & CropDiseases & EuroSAT & ISIC & ChestX \\ \midrule
%     \multirow{2}{*}{1} & LP & \textbf{40.91}{\scriptsize$\pm$.76} & \textbf{73.16}{\scriptsize$\pm$.87} & \textbf{64.96}{\scriptsize$\pm$.86} & 29.80{\scriptsize$\pm$.55} & \textbf{22.32}{\scriptsize$\pm$.42} \\
%      & {FT} & 37.57{\scriptsize$\pm$.70} & 66.82{\scriptsize$\pm$.89} & 57.25{\scriptsize$\pm$.83} & \textbf{31.20}{\scriptsize$\pm$.55} & 22.06{\scriptsize$\pm$.38} \\
%     %  & affinity & 13.45 & 20.91 & 21.12 & 2.69 & 1.32 \\
%     %  & affinity-sub & 57.18 & 44.35 & 56.99 & 17.14 & 11.12 \\
%     \midrule
%     \multirow{2}{*}{5} & LP & 58.38{\scriptsize$\pm$.76} & 91.27{\scriptsize$\pm$.48} & \textbf{84.48}{\scriptsize$\pm$.57} & 40.88{\scriptsize$\pm$.54} & \textbf{26.07}{\scriptsize$\pm$.44} \\
%     & {FT} & \textbf{59.93}{\scriptsize$\pm$.79} & \textbf{91.64}{\scriptsize$\pm$.49} & 82.32{\scriptsize$\pm$.57} & \textbf{48.82}{\scriptsize$\pm$.62} & 25.97{\scriptsize$\pm$.40} \\
%     % & affinity & 19.88 & 13.38 & 28.03 & 0.33 & 3.68 \\
%     % & affinity-sub & 55.97 & 18.30 & 54.00 & 3.12 & 21.32 \\
%     % \midrule
%     % \multirow{2}{*}{10} & LP & 65.31{\scriptsize$\pm$.75} & 94.56{\scriptsize$\pm$.38} & {88.62}{\scriptsize$\pm$.48} & 45.38{\scriptsize$\pm$.54} & {28.88}{\scriptsize$\pm$.43} \\
%     % & {FT} & \textbf{68.68}{\scriptsize$\pm$.74} & \textbf{95.75}{\scriptsize$\pm$.34} & \textbf{88.87}{\scriptsize$\pm$.45} & \textbf{56.11}{\scriptsize$\pm$.61} & \textbf{29.53}{\scriptsize$\pm$.44}\\
%     \midrule
%     \multirow{2}{*}{20} & LP & 71.29{\scriptsize$\pm$.70} & 96.20{\scriptsize$\pm$.29} & 91.00{\scriptsize$\pm$.40} & 51.32{\scriptsize$\pm$.54} & 30.98{\scriptsize$\pm$.45} \\ 
%      & {FT} & \textbf{75.91}{\scriptsize$\pm$.67} & \textbf{97.72}{\scriptsize$\pm$.22} & \textbf{92.54}{\scriptsize$\pm$.36} & \textbf{62.36}{\scriptsize$\pm$.59} & \textbf{32.65}{\scriptsize$\pm$.47} \\
%     %  & affinity & 19.92 & 8.04 & 18.45 & 4.24 & 5.65\\
%     %  & affinity-sub & 41.80 & 9.77 & 27.14 & 10.40 & 27.01 \\
%     \midrule
%     \multicolumn{7}{l}{backbone: ResNet18 pre-trained on tieredIN} \\ \midrule
%     $k$ & Update & miniIN & tieredIN & Places & Plantae & Cars \\ \midrule
%     \multirow{2}{*}{1} & LP & \textbf{63.23}{\scriptsize$\pm$.79} & \textbf{60.38}{\scriptsize$\pm$.93} & \textbf{53.24}{\scriptsize$\pm$.84} & \textbf{38.33}{\scriptsize$\pm$.78} & \textbf{31.86}{\scriptsize$\pm$.59} \\ 
%      & {FT} & 53.42{\scriptsize$\pm$.78} & 52.11{\scriptsize$\pm$.87} & 44.21{\scriptsize$\pm$.73} & 33.10{\scriptsize$\pm$.62} & 30.89{\scriptsize$\pm$.60} \\
%     \midrule
%     \multirow{2}{*}{5} & LP & \textbf{82.95}{\scriptsize$\pm$.49} & \textbf{79.00}{\scriptsize$\pm$.67} & \textbf{72.69}{\scriptsize$\pm$.66} & \textbf{54.78}{\scriptsize$\pm$.84} & 45.91{\scriptsize$\pm$.70} \\ 
%     & {FT} & 79.78{\scriptsize$\pm$.50} & 76.86{\scriptsize$\pm$.70} & 68.33{\scriptsize$\pm$.71} & 52.80{\scriptsize$\pm$.78} & \textbf{47.55}{\scriptsize$\pm$.74} \\
%     % \midrule
%     % \multirow{2}{*}{10} & LP & \textbf{87.06}{\scriptsize$\pm$.41} & \textbf{83.14}{\scriptsize$\pm$.62} & \textbf{77.33}{\scriptsize$\pm$.60} & \textbf{61.03}{\scriptsize$\pm$.81} & 52.92{\scriptsize$\pm$.69}\\ 
%     % & {FT} & 85.70{\scriptsize$\pm$.43} & 82.44{\scriptsize$\pm$.64} & 75.07{\scriptsize$\pm$.65} & 60.12{\scriptsize$\pm$.79} & 55.92{\scriptsize$\pm$.71} \\
%     \midrule
%     \multirow{2}{*}{20} & LP & \textbf{89.12}{\scriptsize$\pm$.34} & 85.90{\scriptsize$\pm$.54} & \textbf{80.50}{\scriptsize$\pm$.54} & 65.38{\scriptsize$\pm$.74} & 58.66{\scriptsize$\pm$.67} \\ 
%      & {FT} & 88.41{\scriptsize$\pm$.37} & \textbf{86.05}{\scriptsize$\pm$.56} & 79.50{\scriptsize$\pm$.57} & \textbf{66.29}{\scriptsize$\pm$.77} & \textbf{62.94}{\scriptsize$\pm$.67} \\
%      \midrule
%     $k$ & Update & CUB & CropDiseases & EuroSAT & ISIC & ChestX\\ \midrule
%     \multirow{2}{*}{1} & LP & \textbf{59.01}{\scriptsize$\pm$.88} & \textbf{66.12}{\scriptsize$\pm$.91} & \textbf{61.95}{\scriptsize$\pm$.89} & 30.53{\scriptsize$\pm$.57} & 21.81{\scriptsize$\pm$.38} \\ 
%      & {FT} & 48.58{\scriptsize$\pm$.80} & 63.61{\scriptsize$\pm$.86} & 54.26{\scriptsize$\pm$.81} & \textbf{31.78}{\scriptsize$\pm$.60} & \textbf{21.92}{\scriptsize$\pm$.37} \\
%     \midrule
%     \multirow{2}{*}{5} & LP & \textbf{77.37}{\scriptsize$\pm$.77} & 86.67{\scriptsize$\pm$.57} & \textbf{80.23}{\scriptsize$\pm$.63} & 42.58{\scriptsize$\pm$.57} & 24.74{\scriptsize$\pm$.42} \\ 
%     & {FT} & 73.99{\scriptsize$\pm$.78} & \textbf{89.52}{\scriptsize$\pm$.51} & 78.96{\scriptsize$\pm$.61} & \textbf{48.45}{\scriptsize$\pm$.61} & \textbf{25.18}{\scriptsize$\pm$.43} \\
%     % \midrule
%     % \multirow{2}{*}{10} & LP & \textbf{82.06}{\scriptsize$\pm$.67} & 90.42{\scriptsize$\pm$.48} & 83.97{\scriptsize$\pm$.55} & 46.15{\scriptsize$\pm$.53} & 26.80{\scriptsize$\pm$.43} \\ 
%     % & {FT} & 80.11{\scriptsize$\pm$.68} & \textbf{94.13}{\scriptsize$\pm$.38} & \textbf{86.36}{\scriptsize$\pm$.50} & \textbf{55.20}{\scriptsize$\pm$.62} & \textbf{27.83}{\scriptsize$\pm$.41} \\
%     \midrule
%     \multirow{2}{*}{20} & LP & \textbf{85.03}{\scriptsize$\pm$.57} & 92.61{\scriptsize$\pm$.41} & 86.30{\scriptsize$\pm$.51} & 50.32{\scriptsize$\pm$.51} & 28.52{\scriptsize$\pm$.41} \\ 
%      & {FT} & 84.30{\scriptsize$\pm$.59} & \textbf{96.33}{\scriptsize$\pm$.28} & \textbf{89.92}{\scriptsize$\pm$.44} & \textbf{60.65}{\scriptsize$\pm$.58} & \textbf{29.86}{\scriptsize$\pm$.44} \\
%      \bottomrule
%     \end{tabular}
%     }
%     \caption{5-way $k$-shot performance according to target dataset.}\label{tab:miniIN_perf}
% \end{table}



% \begin{table}[h!]
% %\vskip 0.10in
% \centering
% \resizebox{\linewidth}{!}{
% \begin{tabular}{clccccc}
%     \toprule
%         {$k$} & {Aug.} & {miniIN} & \!\!\!{CropDiseases}\!\!\! & {EuroSAT} & {ISIC} & {ChestX} \\
%     \midrule
%     \multirow{7}{*}{1} & {-} & 56.23{\scriptsize$\pm$.77} & 73.16{\scriptsize$\pm$.87} & 64.96{\scriptsize$\pm$.86} & 29.80{\scriptsize$\pm$.55} & 22.32{\scriptsize$\pm$.42}\\
%     & {$+$ HFlip} & 56.22{\scriptsize$\pm$.78} & 73.57{\scriptsize$\pm$.88} & 65.14{\scriptsize$\pm$.87} & 29.79{\scriptsize$\pm$.54} & 22.26{\scriptsize$\pm$.41}\\
%     & {$+$ RCrop} & 57.07{\scriptsize$\pm$.79} & 66.10{\scriptsize$\pm$.92} & 66.10{\scriptsize$\pm$.91} & 30.02{\scriptsize$\pm$.55} & 22.10{\scriptsize$\pm$.36}\\
%     & {$+$ CJitter} & 55.90{\scriptsize$\pm$.78} & 72.62{\scriptsize$\pm$.90} & 65.02{\scriptsize$\pm$.86} & 29.80{\scriptsize$\pm$.55} & 22.25{\scriptsize$\pm$.41}\\
%     & {$+$ Base Aug} & 57.28{\scriptsize$\pm$.79} & 66.28{\scriptsize$\pm$.92} & 65.81{\scriptsize$\pm$.92} & 29.82{\scriptsize$\pm$.54} & 22.17{\scriptsize$\pm$.36}\\
%     & {$+$ MixUp} & 51.50{\scriptsize$\pm$.79} & 71.62{\scriptsize$\pm$.88} & 60.38{\scriptsize$\pm$.88} & 29.78{\scriptsize$\pm$.54} & 22.32{\scriptsize$\pm$.41}\\
%     & {$+$ CutMix} & 55.01{\scriptsize$\pm$.79} & 73.31{\scriptsize$\pm$.87} & 64.69{\scriptsize$\pm$.86} & 29.73{\scriptsize$\pm$.55} & 22.41{\scriptsize$\pm$.42}\\
%     \midrule
%     \multirow{7}{*}{5} & {-} & 77.77{\scriptsize$\pm$.61} & 91.27{\scriptsize$\pm$.48} & 84.48{\scriptsize$\pm$.57} & 40.88{\scriptsize$\pm$.54} & 26.07{\scriptsize$\pm$.44}\\
%     & {$+$ HFlip} & 77.84{\scriptsize$\pm$.59} & 91.40{\scriptsize$\pm$.48} & 84.51{\scriptsize$\pm$.58} & 41.11{\scriptsize$\pm$.55} & 26.36{\scriptsize$\pm$.43} \\
%     & {$+$ RCrop} & 77.40{\scriptsize$\pm$.59} & 87.50{\scriptsize$\pm$.56} & 83.43{\scriptsize$\pm$.60} & 41.27{\scriptsize$\pm$.52} & 25.78{\scriptsize$\pm$.42}\\
%     & {$+$ CJitter} & 77.74{\scriptsize$\pm$.61} & 91.08{\scriptsize$\pm$.48} & 84.53{\scriptsize$\pm$.58} & 41.10{\scriptsize$\pm$.54} & 26.28{\scriptsize$\pm$.43}\\
%     & {$+$ Base Aug} & 77.43{\scriptsize$\pm$.59} & 87.17{\scriptsize$\pm$.59} & 83.29{\scriptsize$\pm$.60} & 41.36{\scriptsize$\pm$.52} & 25.66{\scriptsize$\pm$.42} \\
%     & {$+$ MixUp} & 73.45{\scriptsize$\pm$.65} & 90.31{\scriptsize$\pm$.50} & 81.01{\scriptsize$\pm$.61} & 41.38{\scriptsize$\pm$.54} & 25.84{\scriptsize$\pm$.44}\\
%     & {$+$ CutMix} & 75.52{\scriptsize$\pm$.62} & 91.14{\scriptsize$\pm$.47} & 83.55{\scriptsize$\pm$.56} & 40.57{\scriptsize$\pm$.54} & 26.37{\scriptsize$\pm$.43}\\
%     \midrule
%     \multirow{7}{*}{20} & {-} & 86.54{\scriptsize$\pm$.44} & 96.20{\scriptsize$\pm$.29} & 91.00{\scriptsize$\pm$.40} & 51.32{\scriptsize$\pm$.54} & 30.98{\scriptsize$\pm$.45}\\
%     & {$+$ HFlip} & 86.51{\scriptsize$\pm$.44} & 96.20{\scriptsize$\pm$.29} & 91.14{\scriptsize$\pm$.38} & 51.31{\scriptsize$\pm$.53} & 30.97{\scriptsize$\pm$.45} \\
%     & {$+$ RCrop} & 85.65{\scriptsize$\pm$.47} & 93.40{\scriptsize$\pm$.40} & 89.40{\scriptsize$\pm$.44} & 49.52{\scriptsize$\pm$.54} & 30.05{\scriptsize$\pm$.45}\\
%     & {$+$ CJitter} & 86.48{\scriptsize$\pm$.43} & 96.01{\scriptsize$\pm$.30} & 91.17{\scriptsize$\pm$.40} & 51.44{\scriptsize$\pm$.55} & 30.63{\scriptsize$\pm$.47}\\
%     & {$+$ Base Aug} & 85.66{\scriptsize$\pm$.45} & 93.25{\scriptsize$\pm$.40} & 89.46{\scriptsize$\pm$.44} & 49.78{\scriptsize$\pm$.52} & 30.03{\scriptsize$\pm$.43}\\
%     & {$+$ MixUp} & 84.82{\scriptsize$\pm$.47} & 95.40{\scriptsize$\pm$.31} & 88.74{\scriptsize$\pm$.43} & 50.93{\scriptsize$\pm$.54} & 30.07{\scriptsize$\pm$.44}\\
%     & {$+$ CutMix} & 85.67{\scriptsize$\pm$.45} & 95.67{\scriptsize$\pm$.31} & 89.92{\scriptsize$\pm$.42} & 50.01{\scriptsize$\pm$.53} & 30.41{\scriptsize$\pm$.43}\\
%     \bottomrule
% \end{tabular}}
% \caption{5-way $k$-shot performance according to data augmentation techniques. The pre-trained ResNet10 on miniIN is updated.}\label{fig:DA_LP}
% \end{table}
